# Supplementary material for: Clinical Risk Prediction with Temporal Probabilistic Asymmetric Multi-Task Learning
Source: arXiv:2006.12777 source file (2021-02-18)
Supplement: Supplementary file 6 [file Table5.tex]

\begin{table}[ht]
 \footnotesize
 \centering
 \caption{\small Ablation Study - MIMIC-III Infection.} 
  \label{ablation-infection}
 \centering	
 \resizebox{\columnwidth}{!}{
 	\begin{tabular}{cccccc}
 		\toprule
		& \multicolumn{4}{c}{Tasks}       &             \\
		\cmidrule(r){2-5}
		Model  & Fever & Infection & Mortality  & Average \\
		\midrule
		AMTL-intratask 
		& 0.7082 $\pm$ 0.01
		& \textbf{0.7071 $\pm$ 0.01}   
		& 0.6814 $\pm$ 0.03
		& 0.6989 $\pm$ 0.01
		\\
		AMTL-samestep
		& \textbf{0.7130 $\pm$ 0.00}  
		& 0.6946 $\pm$ 0.01 
		& 0.6983 $\pm$ 0.03
		& \textbf{0.7019 $\pm$ 0.01}
		\\
		TD-AMTL      
		& 0.6636 $\pm$ 0.03    
		& 0.6874 $\pm$ 0.01   
		& 0.6953 $\pm$ 0.02 
		& 0.6821 $\pm$ 0.00
		\\
		TP-AMTL (constrained) 
		& \textbf{0.7159 $\pm$ 0.00} 
		& \textbf{0.7003 $\pm$ 0.01}
		& 0.6561 $\pm$ 0.01 
		& 0.6908 $\pm$ 0.00
		\\
		TP-AMTL (epistemic) 
		& 0.6997 $\pm$ 0.01
		& \textbf{0.7196 $\pm$ 0.00} 
		& \textbf{0.7106 $\pm$ 0.02}
		& \textbf{0.7100 $\pm$ 0.01}
		\\
		TP-AMTL (aleatoric) 
		& 0.6984 $\pm$ 0.02    
		& 0.7032 $\pm$ 0.01   
		& \textbf{0.7217 $\pm$ 0.02} 
		& 0.7078 $\pm$ 0.00
		\\
		\midrule
		TP-AMTL (full model)  
		& \textbf{0.7165 $\pm$ 0.00}    
		& \textbf{0.7093 $\pm$ 0.01}   
		& \textbf{0.7098 $\pm$ 0.01} 
		& \textbf{0.7119 $\pm$ 0.00}
		\\
 		\bottomrule
 	\end{tabular}
 }
\end{table}
